# Supplementary material for: A Comprehensive Evaluation of Android ICC Resolution Techniques
Source: arXiv:2111.05649 source file (2022-09-03)
Supplement: Supplementary file 1 [file appendix.tex]

\section{EFSM of Basic Components} ~\label{ap:A}
Fig.~\ref{fig:singleLC} displays the extended finite state machine (EFSM) for the launching of single component, which accepts the executed lifecycle methods of one component.
The lifecycle method inputted into an EFSM will trigger both the changing of EFSM state and the status of a globally maintained component stack $t$.
We use $t(i)$ to denote the $i^{th}$ component from the top in stack $t$. If the current visited component is not in stack $t$, it is represented as $t(0)$.
For example, at state $S_0$, the method \texttt{onCreate()} of a not stored component $t(0)$ will trigger the transition $S_0 \rightarrow S_1$ and component $t(0)$ will be pushed into $t$, i.e., \textit{push} $t(0)$.
After pushing, it can be obtained by getting the top element $t(1)$ from stack.
At state $S_1$, the method \texttt{onStart()} of component $t(1)$ will trigger the transition $S_1 \rightarrow S_2$ and modify the status of component $t(1)$ to \textit{started}, i.e., $t(1).s$ = \textit{started}.
We assume the launch mode of any component is \textit{standard} mode.

\begin{figure}[!htb]
	\setlength{\abovecaptionskip}{5pt}
	\setlength{\belowcaptionskip}{-10pt}
	\centering
	\includegraphics[width=0.42\textwidth]{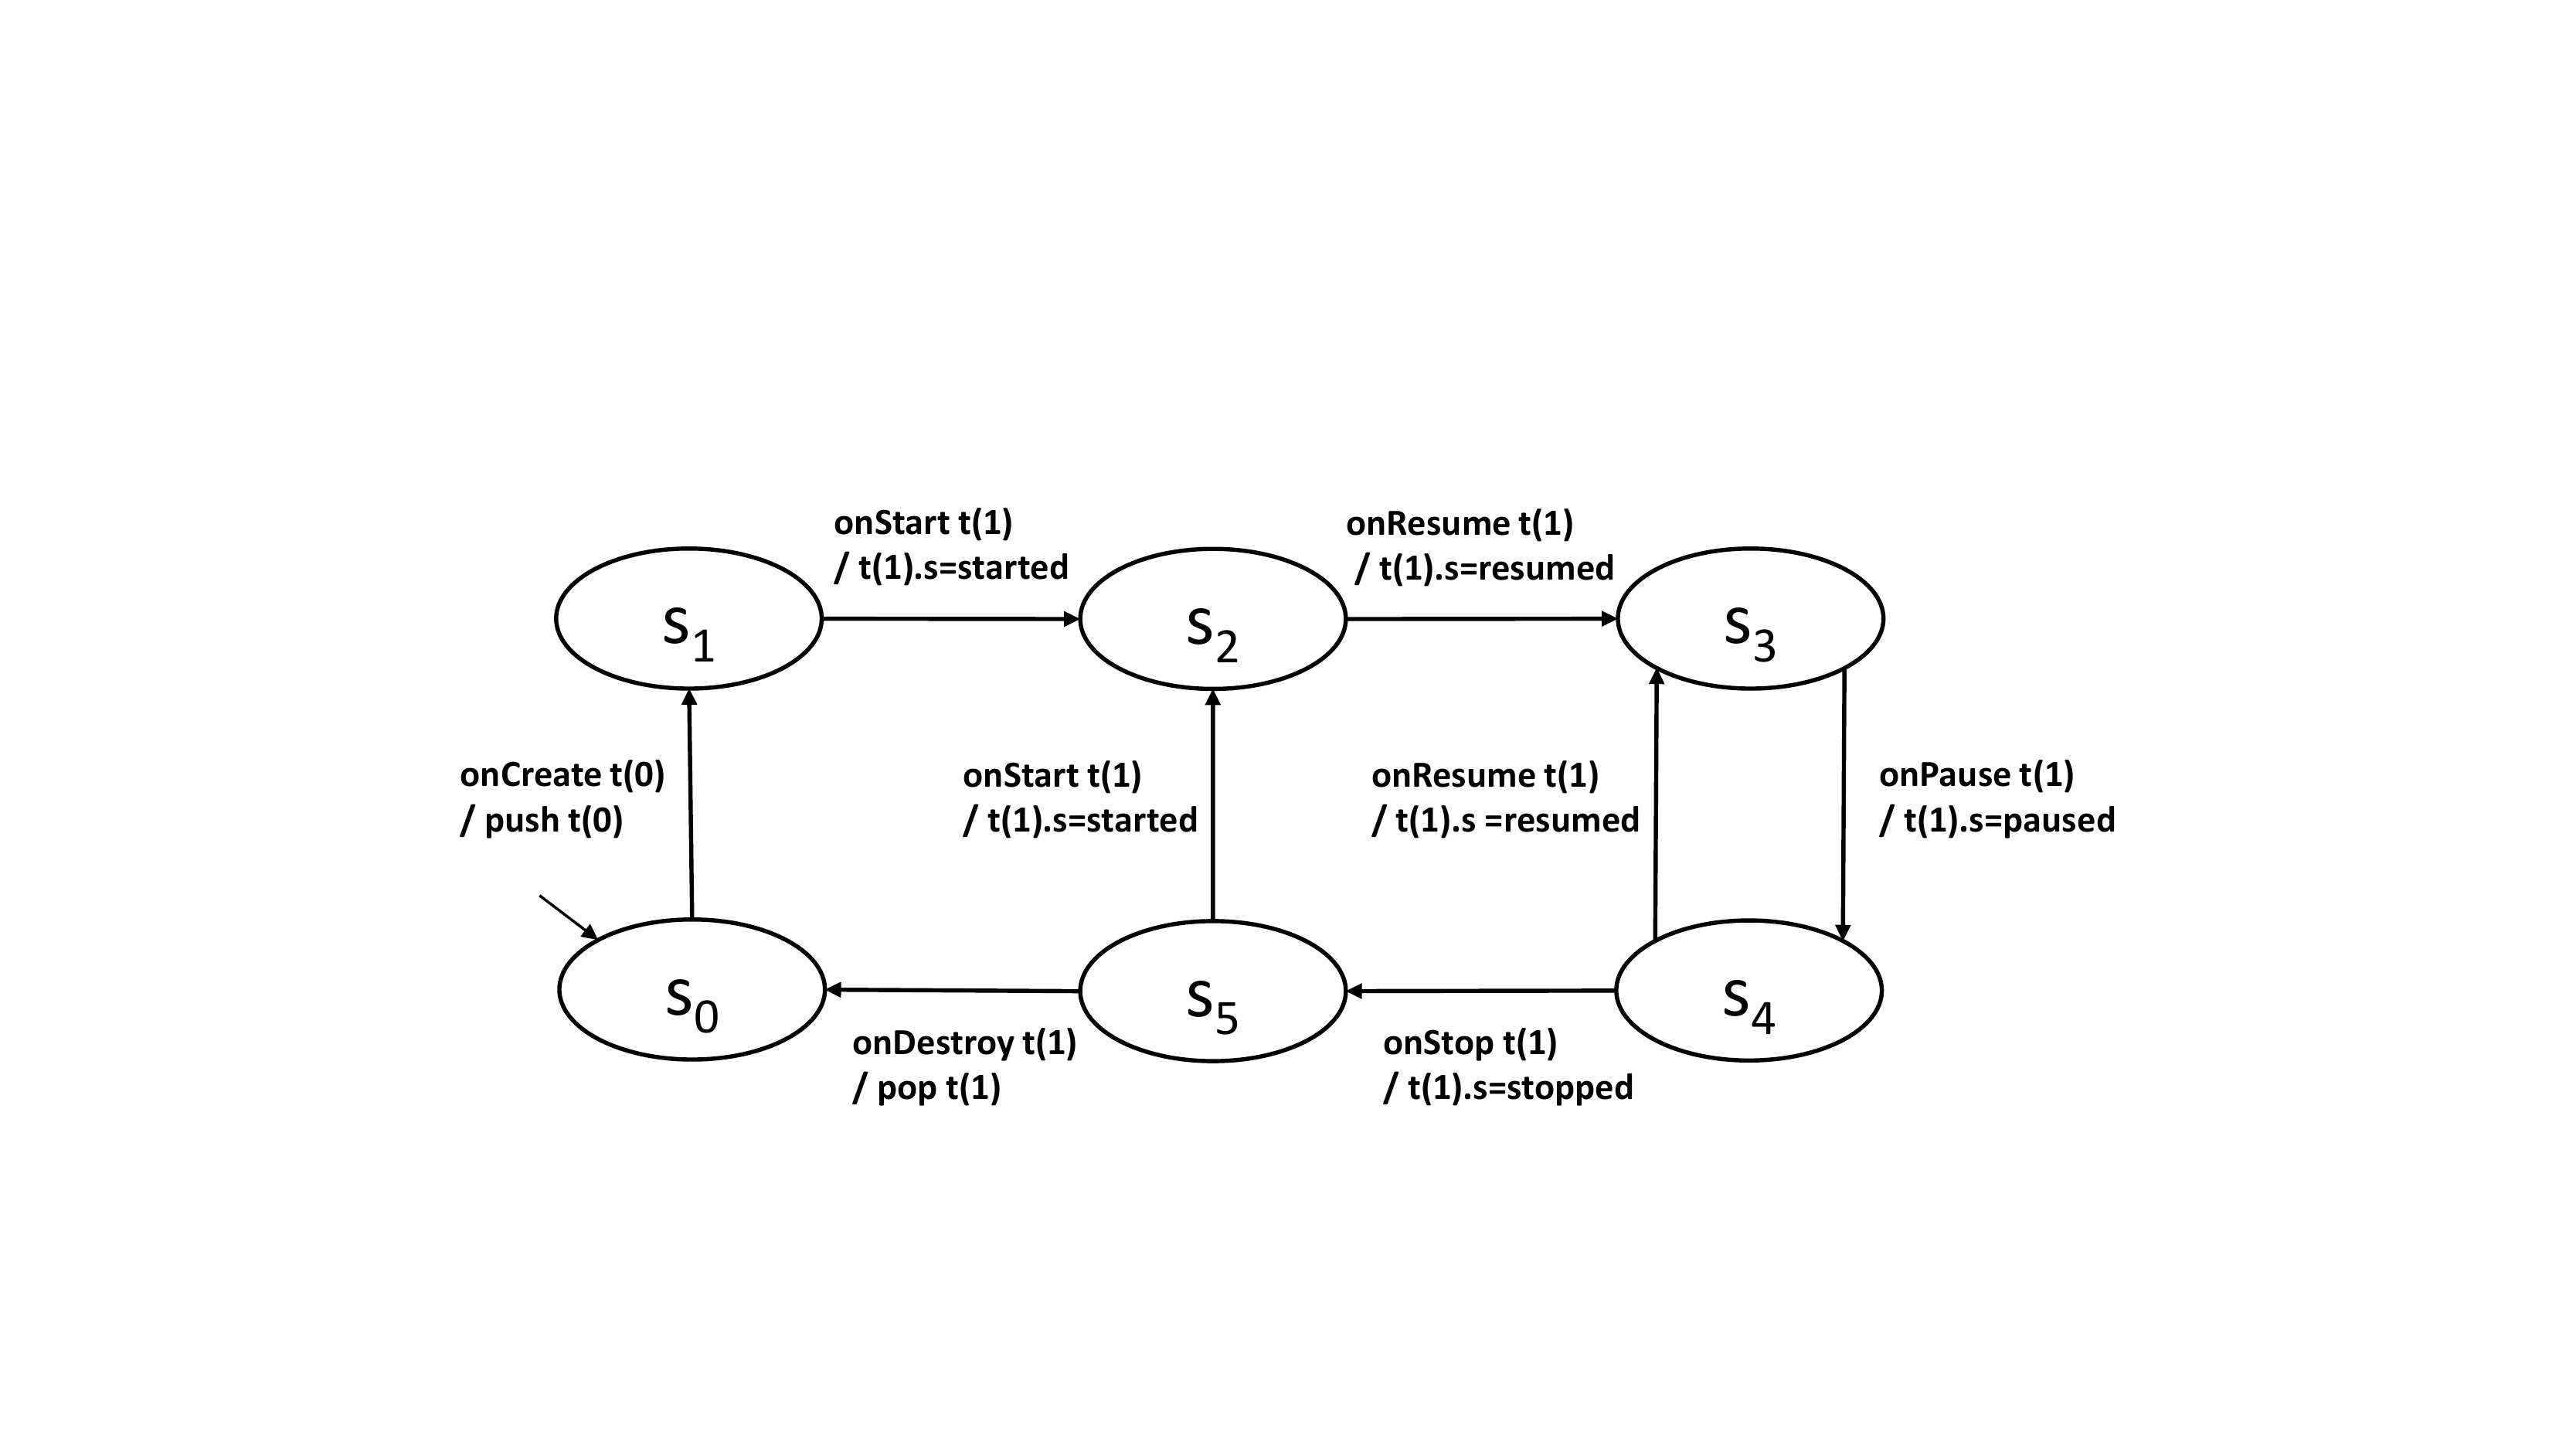}
	\caption{EFSM of Single Component}
	\label{fig:singleLC}
\end{figure}

The EFSM for the launching and interactions of multiple components is given in Fig.~\ref{fig:multipleLC}, in which the red transitions are caused by multiple components interactions. 
For example, if component \textit{A} launch \textit{B}, we get a transition from $s_4 \rightarrow s_1$, then \textit{B} is started and resumed ($s_1 \rightarrow s_2 \rightarrow s_3$). 
After that, the previous component \textit{A} is stopped ($s_3 \rightarrow s_6$), or even destroyed ($s_3 \rightarrow s_6 \rightarrow s_7$).
Another case is that the top component \textit{B} in the stack is going to finish. So, it pauses itself and resumes the previous one ($s_4 \rightarrow s_3$), followed with the component stop and destroys operations ($s_3 \rightarrow s_6 \rightarrow s_7$). In Fig.~\ref{fig:multipleLC}, we merge the transitions with same lifecycle input for simplicity. Note that, the event subsequence (\texttt{onStop} t(1), \texttt{onPause} t(1)) could never happen in reality, as it violates the lifecycle order of single component.

\begin{figure}[hbt!]
	\setlength{\abovecaptionskip}{10pt}
	\setlength{\belowcaptionskip}{-10pt}
	\centering
	\includegraphics[width=0.48\textwidth]{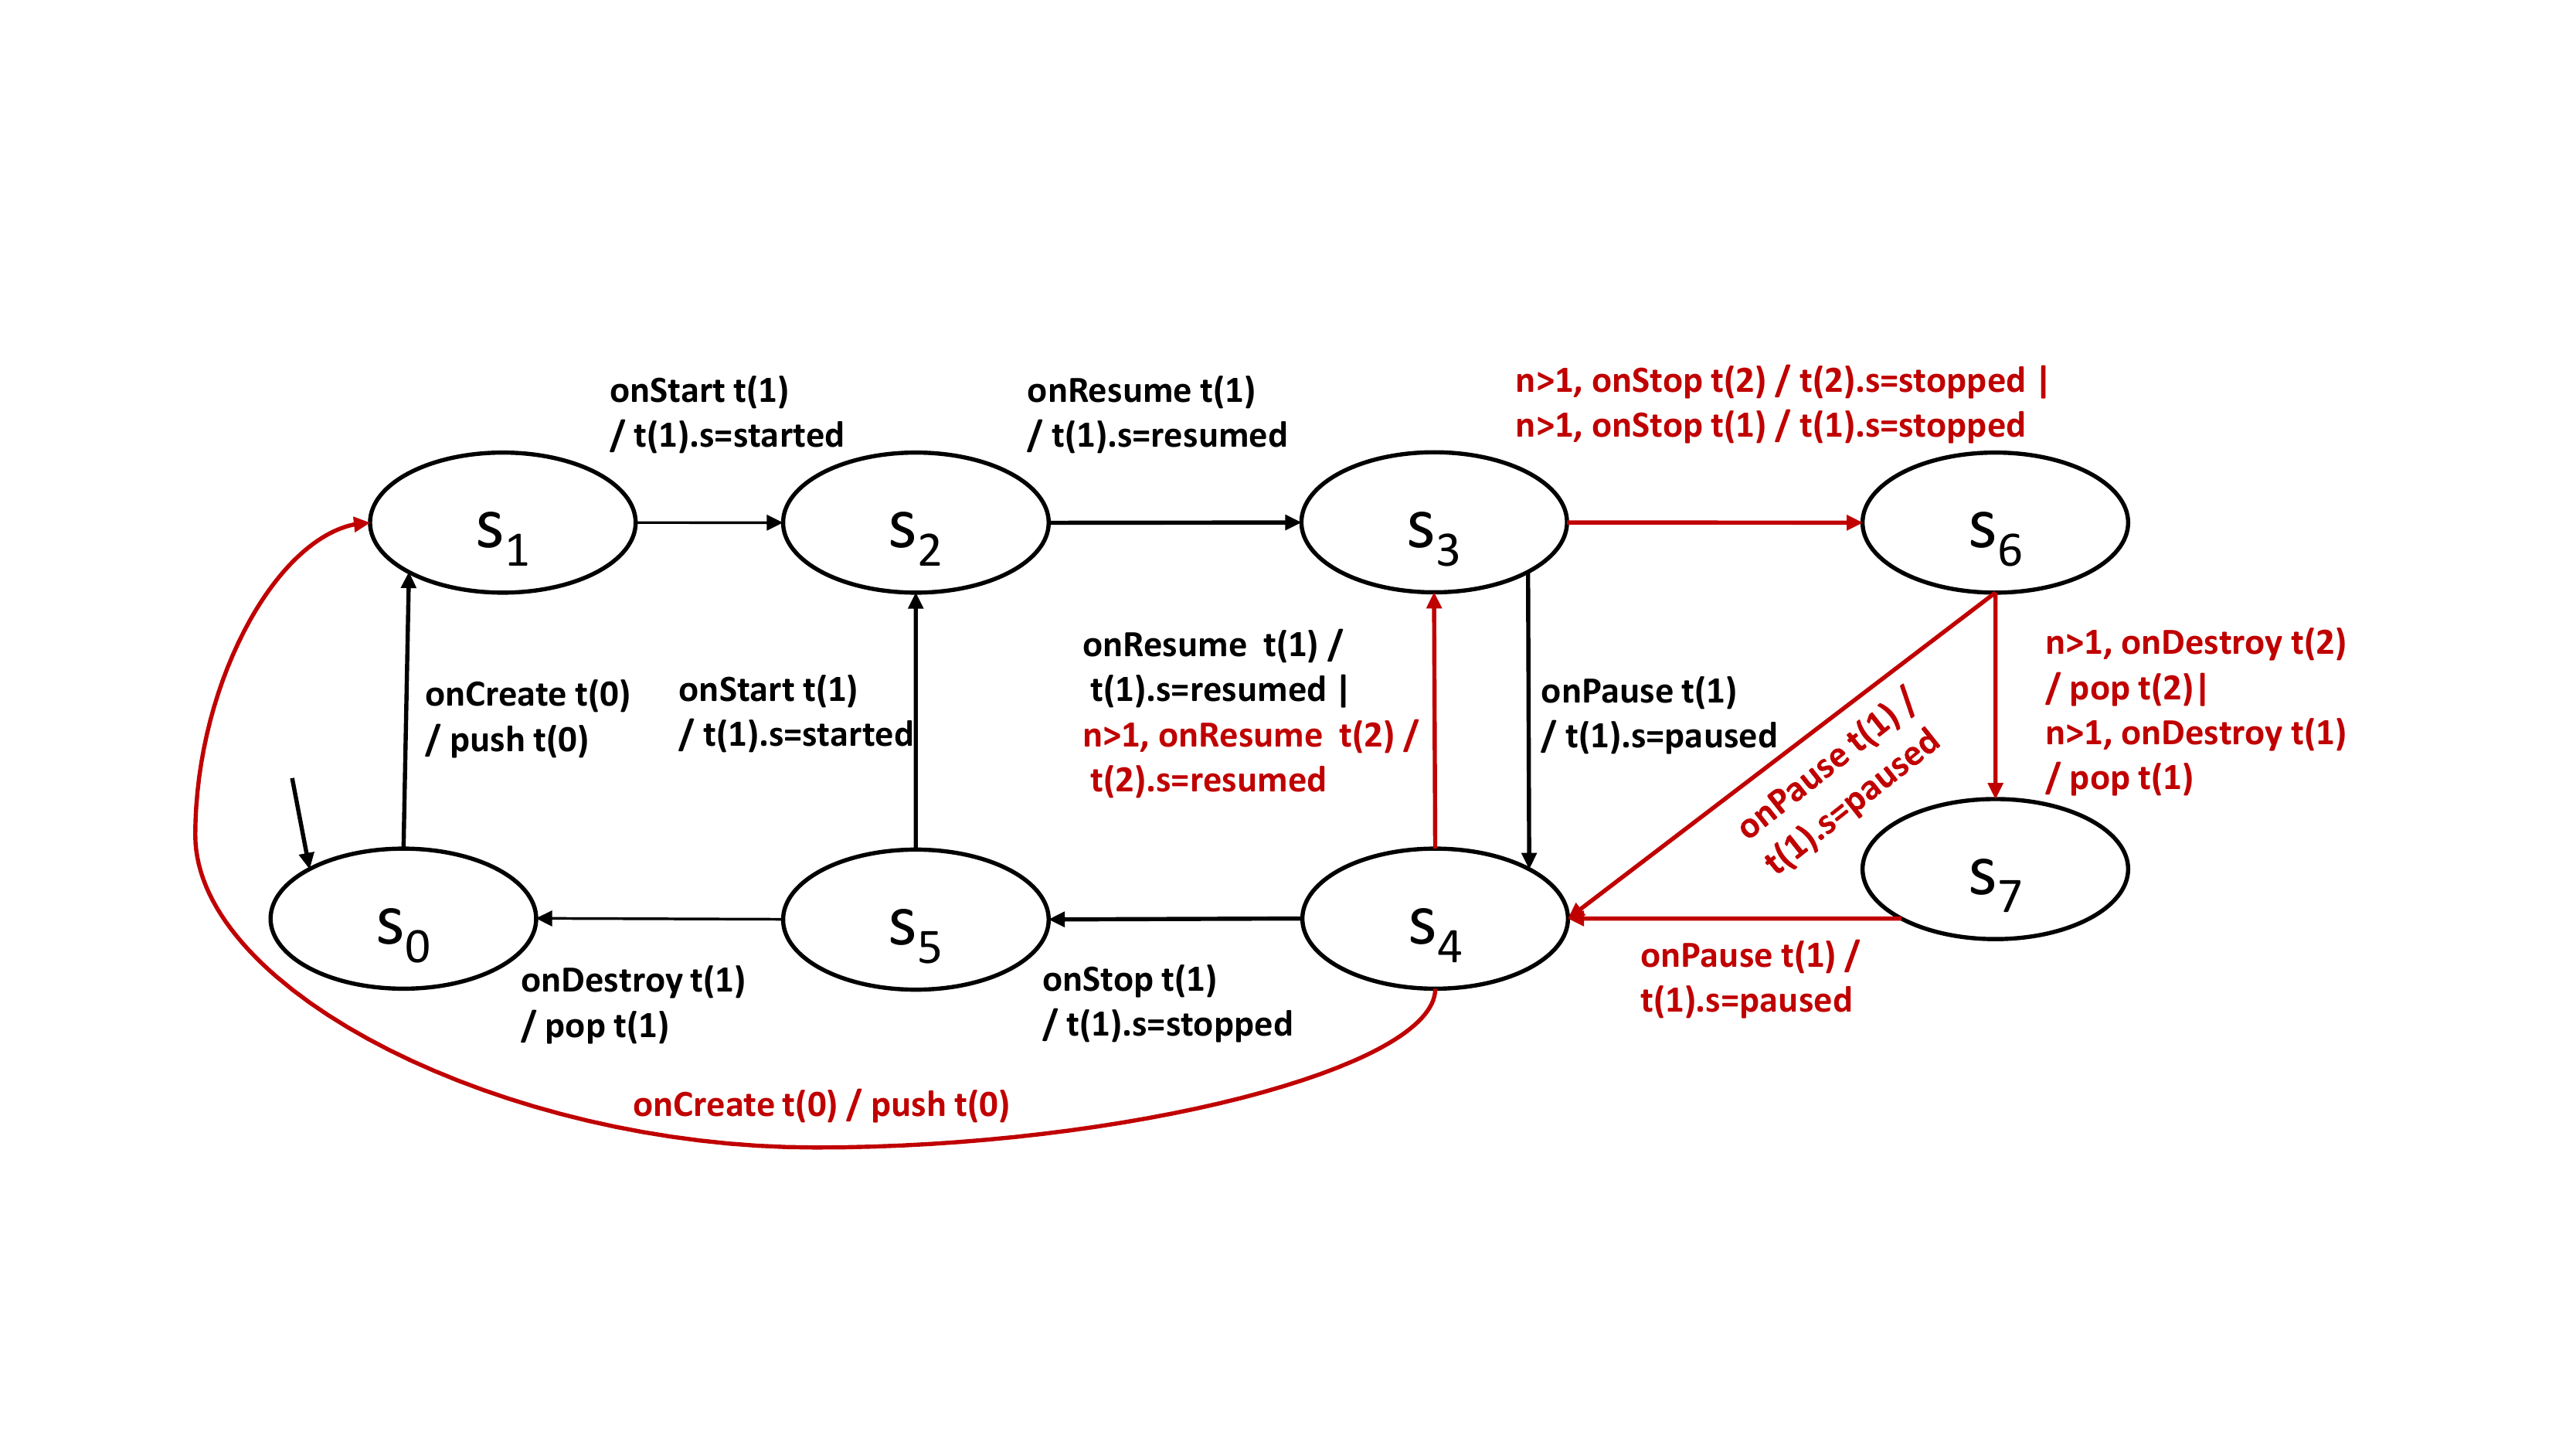}
	\caption{EFSM of Multiple Components}
	\label{fig:multipleLC}
\end{figure}

\section{ICC Extraction Algorithm} ~\label{ap:B}

The ICC extraction algorithm is presented in Algorithm ~\ref{alg:extraction1}.
In line~1, we first preprocess a trace to remove the component switching caused by polymorphic characteristics, e.g, the invocation of \texttt{super.onCreate()}.
In line~2, we build a stack model to store the visited components with a modified stack pushing mechanism.
Considering the incompleteness of lifecycle methods, the callback methods are also concerned, which indirectly denotes the running status of a component.
Among these methods, the stopping related methods, like \texttt{onStop()} and \texttt{onDestroy()}, are excluded as invalid operations, because the execution of them lay back to the methods in the newly launched one (refer to Fig.~\ref{fig:multipleLC}), which confuses the component launching order analysis. 
In lines 5-9, for an executed lifecycle or callback method, if its corresponding component is not in the stack, the component will be pushed into the stack and an ICC link will be reported.
Or else, in lines 11-15, if the corresponding component already exists in the stack, that element will be moved to the top of the stack. In this case, we do not report any new ICC link.
The reason is that a recently visited component is more likely reached by pressing the back button than launched by Intent. 
We adopt a conservative strategy to avoid FP ICCs.
In order to correct the modeling error during analyzing, the stack will be cleared when the default entry component, usually is the \texttt{MainActivity} or the \texttt{SplashActivity}, is revisited and initialized.

\begin{algorithm}[!t]
	\caption{ICC\_extraction\_analysis} \label{alg:extraction1}
	\setlength{\abovecaptionskip}{10pt}
	\setlength{\belowcaptionskip}{-10pt}
	% \small
	\begin{algorithmic}[1]
		\REQUIRE execution trace $trc$, up limit of stack size $k$
		\ENSURE extracted ICC link set $Res$
		\STATE removePolyCall($trc$)
		\STATE $stk$ = new stack()
		\FOR{each ($cpt$, $mtd$) in trace $trc$}
			\IF{$mtd$.isValidLifecycle() or $mtd$.isCallback()}
				\IF{$cpt$ not in $stk$}
					\STATE $stk$.push($cpt$, $mtd$)
					\IF{$stk$.size()>1}
						\STATE $Res$.addICC($stk$.getEle(1), $stk$.getEle(0))
					\ENDIF
				\ELSE
					\FOR{$i$=0; $i$<$stk$.size(); $i$++}
						\IF{$stk$.getEle($i$).equals($cpt$)}
							\STATE  $stk$.moveEletoTop($i$)
						\ENDIF
					\ENDFOR
				\ENDIF
				\IF{$stk$.getEle(0) is the default entry component}
				\STATE $stk$.removeBottom()
				\ENDIF
			\ENDIF
		\ENDFOR
	\end{algorithmic}
\end{algorithm}

For example, if we have a method trace \texttt{A.onCreate()} $\rightarrow$ \texttt{B.onCr\\eate()} $\rightarrow$ \texttt{A.onResume()} $\rightarrow$ \texttt{C.onStart()} $\rightarrow$ \texttt{A.onStop()}.
We first invoke \texttt{removePolyCall()} to filter out the polymorphic call edges. 
If component \texttt{A} extends \texttt{B} and calls \texttt{super.onCreate()}, we remove \texttt{B.onCreate()} in the trace to avoid the FP ICC $A \rightarrow B$ and push \textit{A} into stack.
Or else, ICC $A \rightarrow B$ is extracted, and both \textit{A}, \textit{B} are pushed.
If \textit{B} is in the stack, when method \texttt{A.onResume()} is logged, we take \textit{A} as a back operation leaded transition and do not extract ICC $B \rightarrow A$.
Also, even method \texttt{A.onStop()} shows up later than \texttt{C.onStart()}, we do not report ICC from $C \rightarrow A$ because method \texttt{A.onStop()} is not a valid lifecycle in our approach.
